# Supplementary material for: Encrypted Data Processing
Source: arXiv:2109.09821 source file (2021-09-20)
Supplement: Supplementary file 1 [file AppendixA.tex]

In section foo the data source and the processor or its functional units use a common data encryption/decryption key, shown in blue color in Figure xx., to encrypt the data being sent over an open (unsecured) channel and to decrypt the data received.  This is also referred to as symmetric key or as the “shared secret” in parlance of certain cryptographic protocols.

The class of cryptographic algorithms that use a common encryption/decryption key are called symmetric-key cryptographic algorithms, the prevalent one among them being AES [cite].  The symmetric-key algorithms are much faster than the asymmetric-key algorithms, discussed later in this section, but suffer from three important drawbacks:

\begin{enumerate}
\item
The symmetric key needs to be exchanged over a secure channel.
\item
The identity of the communicating counter-party can not be established.
Non-repudiation of the received messages is not possible.
\end{enumerate}

The asymmetric-key or public-key cryptographic algorithm solve the drawbacks of the symmetric-key algorithms buy allowing for secure exchange of the data encryption key over an open/insecure channel.  To have the best of both worlds, i.e., good encryption/decryption speed and ability to exchange the symmetric key over open/secure channel, cryptography protocols typically use the slower performing asymmetric key cryptography to exchange the symmetric key to be used for data encryption/decryption.  There are two flavors of asymmetric key cryptography

\begin{enumerate}
\item
The symmetric key is chosen by the sender(receiver) encrypted by the public key of the receiver (sender).  The receiver (sender) then uses his private key to obtain the symmetric key.  The quintessential example of this scheme is the RSA (Rivest, Shamir, Adleman) scheme \cite{RSA}.  Among the post quantum cryptography algorithms Kyber uses this approach \cite{Kyber}.
\item
An agreed upon public key (either the sender's or receiver's, or even a universal public key) is used by both the sender or receiver to hash their private keys, and these hashed keys are sent to the counters parties, where the the receiver and sender respectively operate on it with their private key to obtain a shared secret, the symmetric key.  Basically the symmetric key is thus a function of the private keys of both the sender and the receiver, not chosen unilaterally by one of them.
The quintessential example of this scheme, the first to arrive on the assymetric-key cryptography scene is the Diffie Helman key exchange \cite{DiffieHelman76}.
Among the post quantum cryptography algorithms SABER and SIKE use this approach  \cite{SABER, SIDH_std}.
\end{enumerate}. 

In the context of public-key cryptography, we will refer to private-key encrypted by them as message.  The basic elements of public-key encryption algorithm are:
	
% The two communicating parties, Alice and Bob, have their own pair of keys, % 〈A_pub,A_pr 〉 and  〈B_pub,B_pr 〉 respectively.
%	A one-way function E(〖key〗_pub,message)→cypher"_" text.  The key property of this encryption function is that is not easily invertible, i.e., the eavesdropper Eve cannot recover message without the knowledge of 〖key〗_pr, the counterpart of 〖key〗_pub in the 〈〖key〗_pub,〖key〗_pr 〉 pair.
%	A trapdoor function  D(〖key〗_pr,cypher_text)→message, that is easy to compute with the knowledge of 〖key〗_pr.
